# Supplementary material for: Rethinking Data Augmentation for Robust LiDAR Semantic Segmentation in Adverse Weather
Source: arXiv:2407.02286 source file (2024-07-17)
Supplement: Supplementary file 8 [file toyex.tex]

\noindent
\setlength{\tabcolsep}{0.7mm}{
\begin{table}[h]
\centering
\caption{Results of toy experiments from \textit{validation set} of SynLIDAR~\cite{xiao_transfer_2022}.}
\begin{footnotesize}
\scalebox{0.7}{
\begin{tabular}{l|ccccccccccccccccccc|c}
    \toprule
    Methods & \rotatebox{90}{car} & \rotatebox{90}{bi.cle} & \rotatebox{90}{mt.cle} & \rotatebox{90}{truck} & \rotatebox{90}{oth-v.} & \rotatebox{90}{pers.} & \rotatebox{90}{bi.clst} & \rotatebox{90}{mt.clst} & \rotatebox{90}{road} & \rotatebox{90}{parki.} & \rotatebox{90}{sidew.} & \rotatebox{90}{oth-g.} & \rotatebox{90}{build.} & \rotatebox{90}{fence} & \rotatebox{90}{veget.} & \rotatebox{90}{trunk} & \rotatebox{90}{terra.} & \rotatebox{90}{pole} & \rotatebox{90}{traf.} & mIoU \\
    \midrule
    Clean & 0.0 & 54.9 & 94.1 & 0.0 & 0.0 & 94.8 & 93.7 & 0.0 & 94.8 & 0.0 & 89.8 & 0.0 & 98.2 & 53.7 & 76.8 & 90.3 & 0.0 & 86 & 95.2 & 53.8 \\
    \midrule
    \textbf{D1} : soft & 0.0 & 37.0 & 86.7 & 0.0 & 0.0 & 89.5 & 87.8 & 0.0 & 92.6 & 0.0 & 85.1 & 0.0 & 93.8 & 32.4 & 39.5 & 80.9 & 0.0 & 84.7 & 93.0 & 50.2 \\
    \textbf{D1} : hard & 0.0 & 9.1 & 53.9 & 0.0 & 0.0 & 56.0 & 48.6 & 0.0 & 20.9 & 0.0 & 23.7 & 0.0 & 31.0 & 0.4 & 4.8 & 26.7 & 0.0 & 39.6 & 74.4 & \textbf{21.6} \\
    \textbf{D2} : soft & 0.0 & 4.2 & 86.7 & 0.0 & 0.0 & 88.2 & 87.8 & 0.0 & 92.5 & 0.0 & 48.4 & 0.0 & 52.1 & 7.0 & 1.4 & 68.8 & 0.0 & 28.8 & 26.8 & 31.2 \\
    \textbf{D2} : hard & 0.0 & 0.2 & 52.5 & 0.0 & 0.0 & 50.3 & 48.4 & 0.0 & 20.6 & 0.0 & 3.1 & 0.0 & 4.0 & 0.2 & 0.1 & 10.5 & 0.0 & 2.2 & 8.7 & \textbf{11.1} \\
    \textbf{D3} : soft & 0.0 & 55.7 & 79.6 & 0.0 & 0.0 & 86.5 & 87.4 & 0.0 & 45.0 & 0.0 & 50.4 & 0.0 & 55.3 & 22.3 & 6.8 & 74.1 & 0.0 & 69.5 & 29.1 & 34.8 \\
    \textbf{D3} : hard & 0.0 & 12.5 & 11.3 & 0.0 & 0.0 & 63.3 & 32.9 & 0.0 & 0.2 & 0.0 & 3.5 & 0.0 & 6.6 & 1.9 & 2.8 & 45.6 & 0.0 & 4.1 & 0.1 & \textbf{9.7} \\
    \textbf{D4} : soft & 0.0 & 54.8 & 94.1 & 0.0 & 0.0 & 94.8 & 93.8 & 0.0 & 94.8 & 0.0 & 89.8 & 0.0 & 98.2 & 53.8 & 76.6 & 90.2 & 0.0 & 86 & 95.2 & 53.8 \\
    \textbf{D4} : hard & 0.0 & 54.8 & 94.1 & 0.0 & 0.0 & 94.8 & 93.8 & 0.0 & 94.8 & 0.0 & 89.8 & 0.0 & 98.2 & 53.8 & 76.6 & 90.2 & 0.0 & 86 & 95.2 & 53.8 \\
    \bottomrule
\end{tabular}
}
\label{tab:supplementary_toyex}
\end{footnotesize}
\end{table}
